# Supplementary material for: Simulating spin systems with Majorana networks
Source: arXiv:1807.09291 source file (2018-07-24)
Supplement: Supplementary file 1 [file app_ShortChains.tex]

%\documentclass[11pt]{article}
%\usepackage[utf8]{inputenc}
%%\input{headers}
%\input{headers4}
%\usepackage{empheq}
%\DeclareMathAlphabet{\mathpzc}{OT1}{pzc}{m}{it}

\begin{widetext}
{\setstretch{1.3}

\newcommand{\tS}{{\tilde{S}}}
\newcommand{\tm}{{\tilde{m}}}
\newcommand{\cCom}{\mathbin{\raisebox{0.5ex}{,}}}

\section{Groundstate of bipartite Heisenberg systems}\label{app:ChainGroundState}

We review certain groundstate properties of systems with Hamiltonian,
\eq{
H=\sum_{\substack{i\in A\\j\in B}}J_{ij}\S_i\cdot\S_j,
}
where $J_{ij}>0$.
The groundstate is most conveniently described in a rotated basis
\eq{\label{eqn:ZRot}
 \left(\tilde{S}_i^x,\tilde{S}_i^y,\tilde{S}_i^z\right)&=\left(S_i^x,S_i^y,S_i^z\right),\quad i\in A\\
\left(\tilde{S}_j^x,\tilde{S}_j^y,\tilde{S}_j^z\right)&=\left(-S_j^x,-S_j^y,S_j^z\right), \quad j\in B.
}
In terms of the $\tilde{\S}_j$'s, $H$ is
\eq{
H=\sum_{\substack{i\in A\\ j\in B}}J_{ij}\left( \tS^z_i\tS_j^z-\tS_i^x\tS_j^x-\tS_i^y\tS_j^y\right).
}
The Hilbert space, $\mathscr{H}$, is spanned by eigenstates of the $\tilde{S}^z_j$'s:
\eq{
\prod_i\Ket{\tm_i^\a}&=\Ket{\{\tilde{m}_i\}},
&
\tS_i^z\Ket{\tm_i}&=\tm_i\Ket{\tm_i}.
}
Since the total spin-$z$, $\tilde{J}_{tot}^z=\sum_i\tilde{S}_i^z$, commutes with the Hamiltonian, we can divide $\mathcal{H}$ into sectors according to their total $z$-magnetization: 
\eq{
\mathscr{H}&=\bigoplus_M\mathscr{H}^M,
&
\Ket{\{\tm^\a_i\}}=\prod_i\Ket{\tm_i^\a}\in\mathscr{H}^M,
} 
where $\{\tm_i^\a\}$ is a partition of $\tm_i$ such that $M=\sum_i\tm_i^\a$.

The groundstate of $H$ within each $M$-sector satisfy what is known as the ``Marshall sign criterion."
It can be shown that the groundstate of $H$ withitn each $M$-sector is \emph{positive definite} when expressed in the $\Ket{\{\tm_i\}}$ basis:
\eq{
\widetilde{\Ket{gnd;M}}&=\sum_{\{m_i^a\}\in Y^M} f^M_\a\Ket{\{\tm_i^\a\}},\quad f^M_\a>0,
}
where $Y^M$ is the set of \emph{all} partitions $\{m_i^\a\}$ such that $\sum_i m_i^\a=M$.
This is called the ``Marshall sign criterion."
%Here, $\a$ is a sum over \emph{all} partitions with total magnetization in the $z$-direction $M$.
Since there can only be a single state satisfying the sign criterion within any orthogonal set of states, an immediate consequence of having $\widetilde{\Ket{gnd;M}}$ of this form is that it is is non-degenerate (within $\mathscr{H}^M$).

Returning to the original basis, the $M$-sector groundstate is 
\eq{\label{eqn:GndState}
\Ket{gnd;M}_0&=\sum_{\{m_i^a\}\in Y^M} (-)^{\Gamma(\a)}f_\a^M\Ket{\{m_i^\a\}},
&
\Gamma(\a)=\sum_{i\in B}\left({1\o2}+m_i^\a\right).
}
It will be convenient shortly to re-express $\Ket{gnd;M}$ as a sum over states with fixed $z$-magnetizations on the $A$ and $B$ sublattices. 
Assuming $N_A\geq N_B$, we write
\eq{\label{eqn:NewGndState}
\Ket{gnd;M}&=\sum_{m_B=-N_B/2}^{N_B/2}(-)^{{N_B\o2}+m_B}C_{m_B}^M \big|\underbrace{M-m_B}_{m_A},m_B\big>,
&
\Ket{m_A,m_B}&=\sum_{\{m_i^\a\}\in X^M_{m_B}}f_\a^M\Ket{\{m_i^\a\}},
}
where $X_{m_B}^M$ is the set of partitions with $\left(m_A,m_B\right)=\left(M-m_B,m_B\right)$ where $m_{A,B}=\sum_{i\in A,B}m_i^\a$.

%The total spin squared and total spin-$z$ both commute with $H$
%\eq{
%\tilde{J}_{tot}^z=\sum_i\tilde{S}_i^z$.
%}
%The total spin-$z$ operator commutes with $H$. 
%We work in a basis with definite total spin-$z$, $M=\sum_i\tilde{m_i^\a}$.$\tilde{J}_{tot}^z=\sum_i\tilde{S}_i^z$.
%Within 

\subsection{Infinite range Hamiltonian}

We determine the quantum numbers of the groundstate of $H$ by looking at an exactly solvable model, the infinite-range Hamiltonian:
\eq{
H_\infty&=J_\infty\sum_{\substack{i\in A\\ j\in B}}\S_i\cdot\S_j=J\S_{A,tot}\cdot \S_{B,tot}
\nt
&={J_\infty\o2}\left( \J_{tot}^2-\S_{A,tot}^2-\S_{B,tot}^2\right),
}
where $\S_{A,tot}=\sum_{i\in A}\S_i$ and $\S_{B,tot}=\sum_{i \in B}\S_i$.
It's clear that the energy levels depend solely on $\J_{tot}^2$, $\S_{A,tot}^2$, and $\S_{B,tot}^2$ and take the form
\eq{
E\left(j_{tot},s_{A,tot},s_{B,tot}\right)={J_\infty\o2}\left( j_{tot}(j_{tot}+1)-s_{A,tot}(s_{A,tot}+1)-s_{B,tot}(s_{B,tot}+1)\right),
}
where $j_{tot}=\abs{s_{A,tot}-s_{B,tot}},\abs{s_{A,tot}-s_{B,tot}}+1,\dots,s_{A,tot}+s_{B,tot}$.
For a given $(s_{A,tot},s_{B,tot})$, the energy is minimized by setting $j_{tot}=\abs{s_{A,tot}-s_{B,tot}}$.
Assuming $s_{A,tot}\geq s_{B,tot}$, this gives
\eq{
E\left(s_{A,tot}-s_{B,tot},s_{A,tot},s_{B,tot}\right)=-J_\infty s_{A,tot}\left(s_{B,tot}+1\right).
}
It follows that the groundstate of $H_\infty$ is obtained by maximizing $s_{A,tot}$ and $s_{B,tot}$ and letting $j_{tot}=\abs{s_{A,tot}-s_{B,tot}}$.
If there are $N_A$ sites on the A sublattice and $N_B$ sites on the $B$ sublattice, we conclude that the spin quantum numbers of the groundstate are
\eq{
\left(j_{tot},s_{A,tot},s_{B,tot}\right)={1\o2}\left( \abs{N_A-N_B},N_A,N_B\right).
}

\subsection{Quantum numbers of generic bipartite Hamiltonians}

Now let us consider a generic bipartite Hamiltonian $H$ with $N_A$ and $N_B$ sites on the $A$ an $B$ sublattices respectively.
It's clear that within each $M$-sector, the groundstates of both $H$ and $H_\infty$ have definite $j_{tot}$ and satisfy the Marshall sign criterion. 
Let us denote the $M$-sector groundstate of $H$ by $\Ket{M;H}$ and the $M$-sector groundstate of $H_\infty$ by $\Ket{M;\infty}$. 
The Marshall sign criterion then implies that $\Braket{M;H|M;\infty}\neq0$, and we conclude that they have the same total spin: $j_{tot}={1\o2}\abs{N_A-N_B}$.

We can check that this is is consistent with the results presented  in the main text. For the Heisenberg chain with an odd number of sites, one sublattice is larger than the other by a single site; the groundstate therefore has $j_{tot}=1/2$ as claimed.

We also verify our claim in Secs~\ref{sec:MoreBonds} and~\ref{sec:HigherSpins} that the spin configurations in Figs.~\ref{fig:ExtSpins}(b) and (c) have total spin 1 and 3/2 in the groundstate.
For the effective spin-1 site, we have $\left(N_A,N_B\right)=(3,1)$ implying that $j_{tot}={1\o2}\abs{3-1}=1$. 
Similarly, the effective spin-3/2 was constructed with $\left(N_A,N_B\right)=(5,2)$ so that $j_{tot}={1\o2}\abs{5-2}=3/2$.

We can also determine what the minimum number of islands is required in order to obtain an effective spin $j_{tot}$.
Maximizing $j_{tot}$ is equivalent to maximizing the difference is $A$ and $B$ sublattice sites. 
With our set-up, this implies that an effective spin composed of the least number of islands will be in the configuration shown in Fig.~\ref{fig:HigherEffSpin}. 
We see that $N_A=2N_B+1$, meaning that $N_{tot}={1\o3}\left(N_{tot}-1\right)$. 
Since, $j_{tot}={1\o2}\left(N_A-N_B\right)={1\o2}(N_B+1)$, we conclude that at least $N_{tot}=6j_{tot}-1$ islands must be strongly coupled.

%We conclude that the groundstate of any bipartite Hamiltonian $H$ with $N_A=2n$, $N_B=2n+1$ will have a doubly degenerate groundstate manifold with total spin-1/2.
\begin{figure}
\centering
\includegraphics[width=0.98\textwidth]{appendix/HigherEffectiveSpin}
\caption{}
\label{fig:HigherEffSpin}
\end{figure}

\subsection{Projected spins}

In Sec. XX we claimed that the spins of an individual island within an effective vertex are proportional to the total spin operator when projected to the groundstate manifold and that the sign of the proportionality constants altered between sublattices:
 \eq{
\P\S_j\P&=c_j\v{\mathcal{S}},
&
\mathrm{sgn}(c_j)&=\begin{cases}
+1,\quad j\in A
\\
-1,\quad j\in B
\end{cases}
}
where $\P$ projects onto the groundstate manifold of $H$, and $\v{\mathcal{S}}=\P\J_{tot}\P$. 
Here and in what follows, we assume that $N_A> N_B$. 
(As we just saw, when $N_A=N_B$, the groundstate is a singlet and $\Braket{0|\J_{tot}|0}=0$.)

We start by discussing the basis for the groundstate manifold given in Eq.~\eqref{eqn:GndState}.
In particular, we note that the alternating sign convention, $\Gamma(\a)=\sum_{i\in B}\left({1\o2}+m_i^\a\right)$, was chose arbitrarily. 
We could easily have performed the transformation in Eq.~\eqref{eqn:ZRot} on the $A$ sublattice and arrived at the groundstates
\eq{
\Ket{M}'&= \sum_\a(-)^{\tilde{\Gamma}(\a)}\Ket{\{m_i^\a\}}=(-1)^{{1\o2}\left(N_A+N_B\right)+M}\Ket{M},
\nt
\tilde{\Gamma}(\a)&=\sum_{i\in A}\left({1\o2}+m_i^\a\right).
}

The primary consequence of choosing $\Ket{M}$ or $\Ket{M}'$ is that $J_{tot}^\pm$ acts with a different on one or the other:
\eq{
J_{tot}^\pm\Ket{M}&=\pm\sqrt{j_{tot}(j_{tot}+1)-M(M\pm1)}\Ket{M\pm1},
\nt
J_{tot}^\pm\Ket{M}'&=\mp\sqrt{j_{tot}(j_{tot}+1)-M(M\pm1)}\Ket{M\pm1}',
}
We show that the basis $\{ \Ket{M}\}$ in Eq.~\eqref{eqn:GndState} returns $\Braket{M\pm1|J_{tot}^\pm|M}>0$ when $N_A> N_B$.

%To do so, we rewrite the $M$-sector groundstate as a sum over states with a fixed $m_A$ and $m_B$, $\Ket{m_A,m_B}$:
%\eq{\label{eqn:NewGndState}
%\Ket{M}&=\sum_{m_B=-{N_B/2}}^{N_B/2}(-)^{{N_B\o2}+m_B}C^M_{m_B}\Ket{M-m_B,m_B},
%&
%\Ket{M-m_B,m_B}&=\sum_{\{m_i^\a\}\in X^M_{m_B}}f_\a^M\Ket{\{m_i^a\};M}
%}
%where $X_{m_B}^M$ is the set of partititions such that $\sum_{i\in B}m_i^\a=m_B$ and $\sum_{i\in A}m_i^\a=M-m_B$.
We use the expression given in Eq.~\eqref{eqn:NewGndState} to describe the action of $J_{tot}^-=S^-_{A,tot}+S^-_{B,tot}$ on $\Ket{M}$ where $M>-j_{tot}$.
Let us denote the action of $S_{A,tot}^-$ on $\Ket{M-m_B,m_B}$ by
\eq{
S_{A,tot}^-\Ket{M-m_B,m_B}&=
\sum_{\{m_i^\a\}\in X^M_{m_B}}f_\a^M\sum_{i\in A}\sqrt{{3\o4}-m_i^\a(m_i^\a-1)}\Ket{\{m_1^\a,\dots,m_i^\a-1,\dots\}}
\nt
&=\Ket{M-1-m_B,m_B;A^-}\in \mathscr{H}^{M-1}.
}
Similarly, $S_{B,tot}$ acts as
\eq{
S_{B,tot}^-\Ket{M-m_B,m_B}&=
\sum_{\{m_i^\a\}\in X^M_{m_B}}f_\a^M\sum_{i\in B}\sqrt{{3\o4}-m_i^\a(m_i^\a-1)}\Ket{\{m_1^\a,\dots,m_i^\a-1,\dots\}}
\nt
&=\Ket{M-m_B,m_B-1;B^-}\in \mathscr{H}^{M-1}.
}
Note that in the $\big\{\Ket{\{m_i\}}\big\}$ basis, both $\Ket{M-m_B,m_B-1;A^-}$ and $\Ket{M-m_B,m_B;B^-}$ are linear combinations containing only \emph{positive} coefficients over a subset of the states in $\mathscr{H}^{M-1}$. 
With this representation, the action of $J_{tot}^-$ on the state in Eq.~\eqref{eqn:NewGndState} returns
\eq{
J_{tot}^-\Ket{M}&=
\sum_{m_B=-N_B/2}^{N_B/2-1}(-)^{{N_B\o2}+m_B}\left(C_{m_B}^{M}\Ket{M-m_B-1,m_B;A^-}
-C_{m_B+1}^{M}\Ket{M-m_B-1,m_B;B^-}\right)
\nt&\quad
+(-1)^{N_B}C_{N_B/2}^{M}\Ket{M-1-{N_B\o2}\cCom{N_B\o2};A^-}.
}
%Here, we assume that $-j_{tot}<M$.
To determine the sign of $\Braket{M-1|J_{tot}^-|M}$, we focus on the single state in the sum with $(m_A,m_B)=(M-1-N_B/2,N_B/2)$. 
Comparing with the representation of $\Ket{M-1}$ in Eq.~\eqref{eqn:NewGndState}, we conclude that
\eq{
(-1)^{N_B}C_{N_B/2}^{M-1}\Ket{M-1-{N_B\o2}\cCom{N_B\o2}}=\pm(-1)^{N_B}C_{N_B/2}^M\sqrt{j_{tot}(j_{tot}+1)-M(M-1)}\Ket{M-1-{N_B\o2}\cCom{N_B\o2};A^-}.
}
Further, the positivity of $\Ket{M-m_B,m_B-1;A^-}$ guarantees that 
\eq{
\Braket{M-1-{N_B\o2}\cCom {N_B\o2}|M-1-{N_B\o2}\cCom {N_B\o2};A^-}>0,
}
and it follows that the inner product of the states with $-{N_B\o2}\leq m_B<{N_B\o2}$ must also be positive:
\eq{
0<C_{m_B}^M&\Braket{M-1-m_B,m_B|M-1-m_B,m_B;A^-}
\nt&
+C_{m_B+1}^M\Braket{M-1-m_B,m_B|M-1-m_B,m_B;B^-}.
}
Hence, when $N_A> N_B$, $\Braket{M-1|J_{tot}^-|M}>0$. It clearly follows that $\Braket{M+1|J_{tot}^+|M}>0$ as well.

We now show that $\P\S_i\P\,\propto \,\v{\mathcal{S}}$.
The projector is simply given by the outer products of the states in Eq.~\eqref{eqn:GndState}:
\eq{
\P=\sum_{M=-j_{tot}}^{j_{tot}}\Ket{M}\Bra{M}
}
%In what follows, we drop the ``$gnd$" and simply write $\Ket{M}$.
The action of $S_j^z$ on \emph{any} state within the $M$-sector, $\mathscr{H}^M$, will remain in that sector.
In particular, when acting on the state $\Ket{M}$:
\eq{
S_j^z\Ket{M}=\sum_{\{m_i^\a\}\in Y^M} (-)^{\Gamma(\a)} f_\a^Mm_j^\a\Ket{\{m_i^\a\}}\in \mathscr{H}^M.
}
Conversely, the lowering (raising) operator maps states in $\mathscr{H}^M$ to states in $\mathscr{H}^{M-1}$ ($\mathscr{H}^{M+1}$):
\eq{
S_j^\pm\Ket{M}&=\sum_{\{m_i^\a\}\in Y^M}(-)^{\Gamma(\a)}f_\a^M \,\sqrt{{3\o4}-m_j^\a\left(m_j^\a\pm1\right)}\Ket{\{m_1^\a,\dots,m_j^\a\pm 1,\dots\}}\in\mathscr{H}^{M\pm1}.
}
We conclude that
\eq{
\Braket{M'|S_j^z|M}&=a_{j,M}^{(z)}\d_{M',M},
&\Braket{M'|S_j^+|M}&=a_{j,M}^{(+)}\d_{M',M+1},
&
\Braket{M'|S_j^-|M}&=a_{j,M}^{(-)}\d_{M',M-1},
}
where $a_{j,M}^{(z),(\pm)}$ are real numbers.
Next, we note that the identities commutation relations
\eq{
\[S_k^z,J_{tot}^\pm\]&=\pm S_j^\pm,
&
\[J_{tot}^\pm,S_j^\mp\]&=\pm2S_j^z
}
imply the following relations
\eq{
a_{j,M}^{(-)}&=\sqrt{(j_{tot}(j_{tot}+1)-M(M-1)}\left(a_{j,M}^{(z)}-a_{j,M-1}^{(z)}\right),
\nt
a_{j,M}^{(+)}&=\sqrt{j_{tot}(j_{tot}+1)-M(M+1)}\left(a_{j,M+1}^{(z)}-a_{j,M}^{(z)}\right),
\nt
2a_{j,M}^{(z)}&=\sqrt{j_{tot}(j_{tot}+1)-M(M-1)}\,a_{j,M}^{(-)}-\sqrt{j_{tot}(j_{tot}+1)-M(M+1)}\,a_{j,M+1}^{(-)},
\nt
2a_{j,M}^{(z)}&=\sqrt{j_{tot}(j_{tot}+1)-M(M+1)}\,a_{j,M-1}^{(+)}-\sqrt{j_{tot}(j_{tot}+1)-M(M+1)}\,a_{j,M}^{(+)}.
}
Solving we find,
\eq{
a_{j,M}^{(z)}&=Mc_j,
&
a_{j,M}^{(\pm)}&=\sqrt{j_{tot}(j_{tot}+1)-M(M\pm1)}\,c_j,
}
which proves the claim that $\P \S_j\P\,\propto \,\v{\mathcal{S}}.$

Finally, the observation that $c_j>0$ ($c_j<0$) for $j\in A$ ($j\in B$) follows directly from the Marshall sign criterion.
We  use the representation of $\Ket{M}$ in Eq.~\eqref{eqn:NewGndState} to show that $c_j>0$ for $i\in A$:
\eq{
S_j^-\Ket{M}&=\sum_{m_B=-N_B/2}^{N_B/2}(-)^{{N_B\o2}+m_B}C_{m_B}^M\Ket{M-1-m_B,m_B;A_j^-},
}
where the state $\Ket{M-1-m_B,m_B;A_j^-}$ 
is defined to be
\eq{
\Ket{M-1-m_B,m_B;A_j^-}&=S_j^-\Ket{M-1-m_B,m_B;A_j^-}
\nt
&=\sum_{\{m_i^\a\}\in X_{m_B}^M}f_\a^M\sqrt{{3\o4}-m_j^\a(m_j^\a-1)}\Ket{\{m_1^\a,\dots,m_j^\a-1,\dots\}}.
}
As above, $\Ket{M-1-m_B,m_B;A_j^-}$ is a \emph{positive} sum over a subset of the states in $\mathscr{H}^{M-1}$.
Since the sign structure of $S_j^-\Ket{M}$ is the same as for $\Ket{M-1}$, we find
\eq{
\Braket{M-1|S_j^-|M}&=\sum_{m_B=-N_B/2}^{N_B/2}C_{m_B}^{M-1}C_{m_B}^M\Braket{M-1-m_B,m_B|M-1-m_B,m_B;A_j^-}>0,
}
and, hence, that $c_j>0$ as well.

Conversely, acting $S_j^-$ on $\Ket{M}$ \emph{changes} the sign of every state in the sum:
\eq{
S_j^-\Ket{M}&=\sum_{m_B=-N_B/2}^{N_B/2}(-)^{{N_B/2}+m_B}C_{m_B}^MS_j^-\Ket{M-m_B,m_B}
\nt
&=-\sum_{m_B=-N_B/2+1}^{N_B/2}(-)^{{N_B\o2}+m_B}C_{m_B+1}^M\Ket{M-1-m_B,m_B;B_j^-}
}
where we shifted $m_B\to m_B+1$ in the second line, picking up an overall minus sign.
$\Ket{M-1-m_B,m_B;B_j^-}$ is the $B$-sublattice analogue to $\Ket{M-1-m_b,m_b;A_j^-}$, and is therefore also a positive sum over a subset of the states in $\mathscr{H}^{M-1}$.
We conclude that both $\Braket{M-1|S_j^-|M}$ and $c_j$ are less than zero when $j\in B$.

}\end{widetext}
